# Supplementary material for: Predictive Monitoring with Logic-Calibrated Uncertainty for Cyber-Physical Systems
Source: arXiv:2011.00384 source file (2021-07-24)
Supplement: Supplementary file 1 [file appendix.tex]

% example for calculating confidence level
\begin{example}
We show the process of calculating the confidence levels for strong and weak satisfactions in \figref{fig:cf_cfexample}. In \figref{fig:cf_cfexample}(a), we query what confidence level that $\always_{[1,3]}(x_\conflevel>8)$ is strong (left part of the syntax tree) or weak (right part of the syntax tree) satisfied. First, at each time $t \in [1,3]$, we calculate the confidence levels that guarantees the strong satisfaction of $(x_\conflevel>8)$, which are [0,0.38], [0,0.68], [0,0.68]. Next, to calculate $\always_{[1,3]}\phi$, we calculate the intersection of these intervals, which leads to [0,0.38]. 
Similarly, we get the confidence for strong and weak satisfaction of $\always_{[1,3]}(x_\conflevel>10)$ 
in \figref{fig:cf_cfexample}(b), which are [0,0] and [0.38,1], respectively.
% For the weak satisfaction, we can see that 

% Similarly in \figref{fig:cf_cfexample}(b), 
\end{example}

\begin{figure}[t]
\centering
\includegraphics[width=8cm]{Figure/cfexample.png}
\caption{Calculating Confidence Levels} 
% \vspace{-0.3cm}
\label{fig:cf_cfexample}
\end{figure}

\subsection{STL-U Criteria}

Researchers have been applying SRTs to estimate the uncertainty of deep learning models. 
However, for the same deep learning model trained by the same data sets, different SRTs with different parameters will end up with different uncertainty estimation. How to select the SRTs and tune its parameters (i.e, dropout rate $p$) to better capture the model uncertainty is still an open question. In general, most applications just pick a dropout technique and set up its dropout rate by experience without systematically evaluate its influence on the uncertainty estimation. There is a very limited types of criterion on how to train or evaluate the regularization parameters. Accuracy (e.g., RMSE between the real value and mean of the estimated distribution, checking if the real value is within the predicted range) is commonly used as the only metric to evaluate the performance of both deep learning model. For example, as shown in \figref{fig:creterion} (a) and (c), if the ground-truth value $x$ is within the predicted interval $[\lb, \ub]$ (the right figure), it is considered as an accurate uncertainty estimate. Otherwise (the left figure), it is not accurate. The problem of this metric is that it will overestimate the uncertainty, since the larger the uncertain interval is, the more accurate the prediction is. 
For example, comparing \figref{fig:creterion} (a) and (c), if only measuring by accuracy, $(\mathcal{M}_2,p_2)$ expands the predicted interval yet increases the model uncertainty. However, the system will always tend to select $(\mathcal{M}_2,p_2)$ since it has a higher accuracy.

In this paper, we propose a new way to measure the uncertainty interval by checking it against a requirement. As shown in \figref{fig:creterion} (b), the dark area represents a requirement. Obviously, the real value $x$ does not satisfy the requirement. 
Intuitively, when predicting a number, if the real value does not satisfy a requirement, then the estimated interval should also not satisfy the same requirement. However, in \figref{fig:creterion} (b), part of the predicted interval satisfies the requirement, but $x$ could not be within $[\lambda,\ub]$, i.e., this interval is invalid prediction. Therefore, the predicted uncertainty interval should be shorten. As shown in \figref{fig:creterion} (d), the quality of uncertainty interval estimated by $(\mathcal{M}_4,p_4)$ is higher than $(\mathcal{M}_3,p_3)$. In addition,
it is clearer that if the predictive flowpipe satisfies the requirement,
which leads to a higher accuracy on the verification results. Decision makers are easier to tell if the predictive results satisfy the requirement or not.

\begin{figure}[!t]
\centering
\includegraphics[width=0.5\textwidth]{IPSN/Figure_IPSN/criteria_compare.png}
\caption{Comparison of Criteria for Uncertainty Estimation} 
% \vspace{-0.5cm}
\label{fig:creterion}
\end{figure}
